# Supplementary material for: Periodic words, common subsequences and frogs
Source: arXiv:1912.03510 ancillary file (2021-06-04)
Supplement: Supplementary file 1 [file code.pdf]

# Boris Bukh

[Home](#) [Writings](#) [Problems](#) [Teaching](#) [Photos](#) [Contact](#)**Mathematical  
writings**

## Code for "Periodic words, common subsequences and frogs"

### Heuristic algorithm to compute LCS of random words

The usual dynamic programming algorithm to compute the longest common subsequence (LCS) of two words of length  $n$  takes  $\Theta(n^2)$  operations. There exist slightly faster algorithms, the fastest known algorithm still takes  $\Theta(n^2 / \log^2 n)$  operations [3]. However, unless the Strong Exponential Time Hypothesis fails, no algorithm can compute the LCS of a pair of arbitrary words in  $O(n^{2-\delta})$  operations [1].

In our work, we wanted to make numerous computations of the LCS between somewhat long *random* words. In an attempt to take advantage of the fact that our words are not chosen adversarially, we attempted to look only at common subsequences in which only nearby letters are matched. More precisely, given a parameter  $T$ , let  $\text{LCS}_T(V, W)$  be the length of the longest common subsequence between words  $V$  and  $W$  in which the  $i$ 'th letter of  $V$  and the  $j$ 'th letter of  $W$  are never matched unless  $|i - j| \leq T$ . Defining  $T_0 = \lfloor \sqrt{2n} \rfloor$ , and  $T_i = \lfloor \frac{5}{2} T_{i-1} \rfloor$ , we computed  $\text{LCS}_{T_i}$  for  $i = 0, 1, \dots$  in turn, and stopped when two successive computations yielded the same answer.

Since  $\text{LCS}_T$  can be computed in  $\Theta(nT)$  operations using dynamic programming, this is much faster than computing the actual LCS. We ran experiments on many pairs of random words of different lengths.

| $n$       | Number of trials |
|-----------|------------------|
| 2,500     | 300,000          |
| 5,000     | 300,000          |
| 10,000    | 100,000          |
| 20,000    | 40,000           |
| 50,000    | 18,000           |
| 250,000   | 2,600            |
| 500,000   | 1,000            |
| 1,200,000 | 120              |

The two algorithms produced the exact same results each time. Below is the C++11 code used in those experiments. Note that for large values of  $n$ , this code needs a large amount of stack; hence, to avoid segfaults, use `ulimit -s unlimited`.

**windowlcs.cpp**

```
#include <stdio.h>
#include <string.h>
#include <unistd.h>
#include <time.h>
#include "windowlcs.hpp"

const int N=250000;           // Length of the string
const int widthstart=ct_sqrt(2*N); // Initial width
const int Trials=200000;      // Number of trials to perform
const int Verify=1;

// Two random words
symbol A[N];
symbol B[N];

// The next function computes LCS with restriction that symbols farther than width apart are not matched
// It uses the usual recurrence
//   L[i,j]=max(L[i-1,j],L[i,j-1],L[i-1,j-1]+delta_ij)
// but instead of remembering the whole row L[i,...] we remember an array M of size 2width+1
//   L[i,j]=M[j-i+width]
// So, denoting by M' the array corresponding to L[i-1,...] we obtain
```

```

// L[i,j]=max(M'[j+1-i+width],M[j-i-1+width],M'[j-i]+delta_ij)
// That is
// M[d]=max(M'[d+1],M[d-1],M'[d]+delta_{i,i+d-width})
// To avoid treating the first and last values of d separately, we pad the array with initial and final zeros
int computeLCS(const symbol *X, const symbol *Y, int width, int len)
{
    if (width>len)
        width=len;

    int MM[2][2*width+3]; // This array holds both M and M'
    int ind=0;             // MM[ind] is M
    int oind=1;            // MM[oind] is M'
    memset(MM,0,sizeof(MM));
    for(int i=0;i<len;i++)
    {
        for(int d=1;d<2*width+2;d++)
        {
            int j=i+d-(width+1);
            if ((j>=0)&&(j<len)&&(X[i]==Y[j]))
                MM[ind][d]=MM[oind][d]+1;
            else
                MM[ind][d]=max(MM[ind][d-1],MM[oind][d+1]);
        }
        ind=1-ind;
        oind=1-oind;
    }
    return MM[oind][width+1];
}

int errorcount=0;

int computeLCSheuristic(const symbol *X, const symbol *Y, int len, int wstart)
{
    int width=wstart;
    int oldLCS=0;
    int newLCS=0;
    do{
        oldLCS=newLCS;
        width=(width*5)/2;
        newLCS=computeLCS(X,Y,width,len);
    } while (newLCS!=oldLCS);

    // Verify correctness of the heuristic computation
    if (Verify)
        if (newLCS!=computeLCS(X,Y,len,len))
            errorcount++;

    return newLCS;
}

int main()
{
    initRandom();

    time_t lastTime = time(NULL);

    for (int i=1;i<=Trials;i++)
    {
        genRandomBinary(A,N);
    }
}

```

```

    genRandomBinary(B,N);
    computeLCSheuristic(A,B,N,widthstart);
    if ((i % 5 )==0)
    {
        time_t curTime = time(NULL);
        if (difftime(curTime,lastTime)>15)
        {
            lastTime=curTime;
            printf("LCS was computed incorrectly %d times out of %d trials for n=%d.\n",errorcount,i,N);
        }
    }
}

return 0;
}

```

## windowlcs\_helpers.cpp

```

#include <stdio.h>
#include <unistd.h>
#include <fcntl.h>
#include "windowlcs.hpp"

int randomData;

// Initializes a random string of N bits
void genRandomBinary(symbol *W,int len)
{
    unsigned char buf[256];
    int bufpos=0;
    for (int i=0;i<len;i++)
    {
        if(bufpos==0){
            if (read(randomData,buf,256)!=256)
            {
                printf("Ouch!");
                return;
            }
            bufpos=256*8;
        }
        bufpos--;
        int byteno=bufpos/8;
        int bitno=bufpos%8;
        W[i]=(buf[byteno]>>bitno)&1;
    }
}

void initRandom()
{
    randomData = open("/dev/urandom", O_RDONLY);
    if (randomData < 0)
        printf("Failed to open /dev/urandom.\n");
}

```

## windowlcs.hpp

```

#ifndef WINDOWLCSHPP
#define WINDOWLCSHPP
#include <stdint.h>

#define max(a,b) \

```

```

({ __typeof__ (a) _a = (a); \
  __typeof__ (b) _b = (b); \
  _a > _b ? _a : _b; })

#define min(a,b) \
({ __typeof__ (a) _a = (a); \
  __typeof__ (b) _b = (b); \
  _a < _b ? _a : _b; })

#define SQRTMID ((lo + hi + 1) / 2)

constexpr uint64_t sqrt_helper(uint64_t x, uint64_t lo, uint64_t hi)
{
  return lo == hi ? lo : ((x / SQRTMID < SQRTMID)
    ? sqrt_helper(x, lo, SQRTMID - 1) : sqrt_helper(x, SQRTMID, hi));
}

constexpr uint64_t ct_sqrt(uint64_t x)
{
  return sqrt_helper(x, 0, x / 2 + 1);
}

typedef unsigned char symbol;

void initRandom();

// Initializes a random string of len bits
void genRandomBinary(symbol *W, int len);

#endif

```

After writing the paper, we learned from Alex Tiskin that a similar idea was independently proposed by Schimd and Bilardi [4] in the context of Levenshtein distance. Denoting by  $L(V, W)$  the Levenshtein distance between words  $V$  and  $W$ , one may define  $L_T(V, W)$  in a manner similar to how  $\text{LCS}_T(V, W)$  was defined. Schimd and Bilardi computed  $L_T$  for  $T = \sqrt{n}$  and  $n = 2^{20}$  as a way to estimate  $\mathbb{E}_{V,W} L(V, W)$ . To test their approach in the context of the LCS, we computed  $\text{LCS}_{\sqrt{n}}$  for  $n = 2^{20}$  using the code above. Out of 130 random trials, not in a single trial did  $\text{LCS}(V, W)$  and  $\text{LCS}_{\sqrt{n}}(V, W)$  agree.

#### Algorithm to compute LCS between a random word and a periodic word

Let  $W$  be a periodic word, and let  $W^{(n)}$  be the word of length  $n$  obtained by concatenating copies of  $W$ . If  $n$  is not divisible by  $\text{len } W$ , we truncate the last copy appropriately. For example, if  $W = 012$ , then  $W^{(8)} = 01201201$ . In the paper we showed that  $\mathbb{E} \text{LCS}[R, W^{(pn)}] = \gamma_W(\rho)n - O(\sqrt{n})$ , where

$$\gamma_W(\rho) = \rho - \frac{1}{\text{len } W} \sum_{s_m \leq \rho} (\rho - s_m),$$

and  $s_m$  is the speed of  $\mathfrak{S}_m$  in the frog dynamics associated with  $W$ . Below is a program that searches for a word  $W$  with large  $\gamma_W(1)$ , and relies on being able to compute  $\gamma_W$  efficiently. The code can also be used to compute  $\gamma_W$  of a single word  $W$ .

Notable features (and mis-features) of the code:

- To compute the constant  $\gamma_W(\rho)$ , the speeds exceeding  $\rho$  need not be known. The code takes advantage of that and computes no more speeds than necessary.
- If the upper bound is lower than the largest  $\gamma_W(1)$  observed, the code skips to the next word.
- The code was written before all the results in the paper were obtained. If I were to write it now, I would compute the sums

$\Sigma_m = s_1 + \dots + s_m$  for each  $m = 1, 2, \dots$  as in Section 4.1 of the paper.

- The code computes  $s_m - s_{m-1}$  directly. That quantity can be thought as measuring the rate at which  $\Sigma_m$  jumps over  $\Sigma_{m-1}$ . To that end, it uses 'fragments' which encode the part of the  $k$ -height between  $(m-1)$ 'st and  $m$ 'th ledge.
- The fragments are reduced, which means that if the distance between successive ledges is greater than  $k$ , then the repeating part is removed, and the distance is reduced by  $k$ .
- Instead of working with  $k$ -heights directly, the code manipulates *profiles*. For a  $k$ -height  $h$ , the associated profile is  $P(x) = h(x) - h(x-1)$ . Note that there is a bijection between  $k$ -heights and profiles.

**froglcs.cpp**

```
#include <stdlib.h>
#include <stdio.h>
#include <string.h>
#include <stdint.h>
#include <assert.h>
#include <set>
#include <vector>
#include <gmp.h>    // GMP library for rational number arithmetic
#include <gmpxx.h>  // ... and a C++ wrapper for it (for sanity's sake)

// Linear solver
#include <linbox/field/gmp-rational.h>
#include <linbox/solutions/solve.h>
#include <linbox/solutions/methods.h>

const int alphabet=2;                // Alphabet size. The symbols are 0123456789.; etc

char periodicWord[] = "0000000000"; // The program will compute gamma_W(1) for all W in
                                     // the lexicographic order starting from this word
                                     // (it will avoid re-computing gamma_W(1) for words
                                     // that differ only in a cyclic shift or reversal)

// If you are interested in computing gamma_W(1) for just for a single word and do not wish to modify the code,
// then set periodicWord[] accordingly, and abort the program after it computes gamma_W for that word

// If you are interested in computing gamma_W(rho) for some other rho, change the first line of
// estimateExpectedLCS() below

// Should we test only balanced words (those with equally many of each symbol)
// Emprically, the words with largest gamma_W are balanced
const bool balancedOnly = false;

// Compute period at compile time
#define STRLEN(s) ((sizeof(s)/sizeof(s[0]))-1)
static const int k = STRLEN(periodicWord);

typedef unsigned long profile;        // Profiles stored as bitmasks
#define profilePopcount __builtin_popcountl // How many 1 bits are there?
const profile allOneProfileMask=(1ul<<k)-1ul; // All-1 mask

typedef int state_t;
typedef std::set <state_t, std::greater <state_t> > stateSet;

void printProfile(profile P, bool newline=false, int minwidth = 1)
{
    int width=0;
    while (P!=0)
```

```

    {
        printf("%d", (int) (P%2));
        P=P/2;
        width++;
        if(width==k)
            printf(" ");
    }
    while (width++ < minwidth)
        printf(width==k ? "0 " : "0");
    if(newline)
        printf("\n");
}

// Starting at profile P, poke frogs at lilypads indexed by bitmask I.
// The bitmask must be periodic with period k. Returns the resulting profile.

profile poke(profile P, profile I)
{
    // pseudocode
    // k=0
    // do
    //     if I[k]==1 && P[k]==0
    //         P[k]=1
    //         k++
    //     while P[k]==0
    //         k++
    //         P[k]=0
    //         k++
    //
    // We use bit-twiddling to achieve the same purpose
    // (note that we use that unsigned integer types do not under/overflow and just wrap around mod 2^whatever)
    // Example (bit are from least significant to most significant)
    //     P = 000010001..
    //     I = 01xyz01wq..
    //     I&(~P) = 01xy001w0..
    //     P-I&(~P) = 01XY001W0.. (where x is complement of X, y is complement of Y,...)
    //     I&(P-I&(~P)) = 010000100..

    //     P = 000010001001..
    //     I = 01xyz01wq000..
    //     I&(~P) = 01xy001w0000..
    //     P-I&(~P) = 01XY001W0001.. (where x is complement of X, y is complement of Y,...)
    //     I&(P-I&(~P)) = 010000100000..
    //     P&(P-I&(~P)) = 000000000001

    return (P-(I&(~P)))&(I|P);
}

profile Is[alphabet];

// takes a bitmask of k bits, and concatenates it with it itself to obtain bitmask suitable for use in poke()
profile makePeriodic(profile I)
{
    profile prev;
    profile res=I;
    do {
        prev=res;
        res=(prev<<k)|I;
    }

```

```

    } while (res!=prev);
    return res;
}

void initIs(const char *s)
{
    assert(k==strlen(s));
    memset(Is,0,sizeof(Is));
    for (int p=0;p<k;p++)
    {
        int v=s[p]-'0';
        Is[v]|=1<<p;
    }
    for (int c=0;c<alphabet;c++)
        Is[c]=makePeriodic(Is[c]);
}

// A "fragment" is a data structure that describes the profile between two successive ledges.
// Below we assume that we are interested in what happens between k-y'th and k-y+1'st ledge.
// The fragment is stored in a 2*k bit string with the following format.
// First k bits:
//     The first k bits end with a 0
//     The first k bits contain exactly k-y 0's
// Last k bits:
//     If there is an 0 in i'th position, then there is a 0 in k+i'th position
//     The remaining y-k positions among last k bits are of the form 1111000

// Note that in order to know the effect of a poke on a fragment, we must keep track of the
// position mod k of where the ledge is; that is the "shift" parameter below

// Poke fragment
//   boolean emit is set to true if we emit a [1:y] option (i.e. the k-y+1'st frog jumps over k-y'th)
//   increment shift by the number of bits shifted (and reduce mod k at the end)
profile pokeFragment(profile F, profile I, int y, int &shift, bool &emit)
{
    profile P=poke(F,I);
    while (profilePopcount(P&allOneProfileMask)>y)
    {
        P>>=1;
        shift=(shift+1)%k;
    }
    if ((profilePopcount((P>>k)&allOneProfileMask))==y)
    {
        emit=true;
        return P&allOneProfileMask;
    }

    emit = false;
    // set extra 1's to zero
    // For example if k=4, and P=11101010 then we want to emit 11101000
    profile First = P & allOneProfileMask;
    profile Last = (P>>k)&allOneProfileMask;

    // Locate the first 1 bit in First&(~Last) and set all the bits after that to 0
    profile A = First&(~Last);
    return ((Last&(A^(A-1)))<<k)|First;
}

// makes fragment whose first k bits are First

```

```

// and of weight s in the last k bits
profile makeFragment(profile First, int s)
{
    profile Last=0;
    int i=0;
    int j=0;
    while(i<s)
    {
        while (((1<<j)&First)==0)
            j++;
        Last|=1<<j;
        i++;
        j++;
    }
    return (Last<<k)|First;
}

// Compute the binomial coefficients
// Copied from https://stackoverflow.com/questions/24294192/computing-the-binomial-coefficient-in-c
int binom(int n,int k)
{
    assert(n>=k);
    assert(k>=0);
    int ans=1;
    k=k>n-k?n-k:k;
    int j=1;
    for(;j<=k;j++,n--)
    {
        if(n%j==0)
        {
            ans*=n/j;
        }else
        if(ans%j==0)
        {
            ans=ans/j*n;
        }else
        {
            ans=(ans*n)/j;
        }
    }
    return ans;
}

// The states of our Markov chain will be the fragments.
// The following arrays will store the states. The index is the shift parameter.
int possibleCount[k];
profile *possibleFragments[k];

int compareProfile(const void *elem1, const void *elem2)
{
    int f = *((profile*)elem1);
    int s = *((profile*)elem2);
    return (f>s) - (f<s);
}

// Compute all possible fragments, and sort them
void computePossibleFragments(int y)
{
    assert(y<k);

```



```

// Possible tuples of first k bits are binom(k-1,k-y-1) in number
// For each of them the number of 1's among last k bits is between 0 to y-1

possibleCount[y] = binom(k-1,k-y-1)*y;
possibleFragments[y] = (profile*) malloc(sizeof(profile)*possibleCount[y]);

int cnt=0;
for(profile First=0;First<=(allOneProfileMask>>1);First++)
    if (profilePopcount(First)==y)
        for(int s=0;s<y;s++)
            possibleFragments[y][cnt++]=makeFragment(First,s);

qsort(possibleFragments[y],possibleCount[y],sizeof(profile),compareProfile);
assert(cnt==possibleCount[y]);
}

// looks for fragment in y'th fragment array (binary search)
int findFragment(int y, profile F)
{
    // We narrow to half-open interval [L,R)
    int L=0;
    int R=possibleCount[y];
    while (L<R)
    {
        int M=(L+R)/2;
        if (F>possibleFragments[y][M])
            L=M+1;
        else if (F<possibleFragments[y][M])
            R=M;
        else
        {
            assert(F==possibleFragments[y][M]);
            return M;
        }
    }
    assert(false);
    return -1;
}

// a state consists of a Fragment and a shift
// we encode it in a number X s.t. X%k is the shift
// and X/k is the index of the fragment in the appropriate possibleFragments[..] array

// This function computes the result of applying symbol c to a given state
state_t transition(int y,state_t state,int c,bool &emit)
{
    state_t ind=state/k;
    int shift=state%k;
    int F=pokeFragment(possibleFragments[y][ind],Is[c]>>shift,y,shift,emit);
    return findFragment(y,F)*k+shift;
}

void printState(int y,state_t state)
{
    state_t ind=state/k;
    int shift=state%k;
    printProfile(possibleFragments[y][ind],false,2*k);
}

```

```

    printf("{%d}", shift);
}

// maxStates = max_y binom(k-1, k-y-1) * y * k
// I would be happy to compute max_y binom(k-1, k-y-1) * y * k at compile time
// but using -std=c++11 option in order to use constexpr causes lots of errors
// when including the standard headers
//
// I wish I could use binom(n, x) <= 2^n / Sqrt[Pi n/2] but alas sqrt() is not considered constexpr either (ouch!)
//
// So, we just boringly precompute the constants :-(

static const int maxStatesTable[] =
    {0, 0, 2, 6, 24, 60, 180, 420, 1120, 2520, 6300, 13860, 33264, 72072, 168168, 360360, 823680, 1750320, 3938220};
static const int maxStates = maxStatesTable[k];

typedef int stateTransition[k];

int stateCount;
state_t feasibleStates[maxStates];
stateTransition stateTransitions[maxStates];
stateTransition transitionEmissions[maxStates];

// This array will hold the stationary distribution
mpq_class prob[maxStates];

// looks for state in feasibleState array (binary search)
int findFeasibleState(state_t S)
{
    // We narrow to half-open interval [L, R)
    int L=0;
    int R=stateCount;
    while (L<R)
    {
        int M=(L+R)/2;
        if (S>feasibleStates[M])
            L=M+1;
        else if (S<feasibleStates[M])
            R=M;
        else
        {
            assert(S==feasibleStates[M]);
            return M;
        }
    }
    assert(false);
    return -1;
}

void computeTransitions(int y)
{
    assert(y>0);
    assert(y<k);
    stateSet processed, unprocessed;
    unprocessed.insert(0);
    while (!unprocessed.empty())
    {

```

```

    state_t S=*unprocessed.begin();
    for(int c=0;c<alphabet;c++)
    {
        bool emit;
        profile Snext = transition(y,S,c,emit);
        if ((unprocessed.count(Snext)==0)&&(processed.count(Snext)==0))
            unprocessed.insert(Snext);
    }
    unprocessed.erase(S);
    processed.insert(S);
}

stateCount = 0;
for (stateSet::reverse_iterator itr = processed.rbegin(); itr!=processed.rend(); ++itr)
    feasibleStates[stateCount++]=*itr;
for(int i=0;i<stateCount;i++)
{
    for(int c=0;c<alphabet;c++)
    {
        bool emit;
        state_t Snext=transition(y,feasibleStates[i],c,emit);
        transitionEmissions[i][c]=emit;
        stateTransitions[i][c]=findFeasibleState(Snext);
    }
}
}

typedef LinBox::GMPRationalField LinBoxField;

void computeStationaryDistribution()
{
    typedef LinBoxField Field;
    typedef LinBox::SparseMatrix<Field> Matrix;
    Field F;
    typedef std::vector<Field::Element> Vector;

    Matrix AL(F,stateCount,stateCount);
    Vector BL(stateCount);
    Vector Res(stateCount);

    // Set up vector and matrices

    // B=[0,0,...,0,1]
    F.init(BL[stateCount-1],1);

    // For 0<=i<stateCount-1 the i'th row of A expresses that
    // i'th element of solution vector is the stationary distribution of i'th state
    // (note that we skip the condition for last state because of linear dependence)
    //
    // The last row of A says that the sum of probabilities is 1

    // Diagonal
    Field::Element v;
    F.init(v,-alphabet);
    for(int i=0;i<stateCount-1;i++)
        AL.setEntry(i,i,v);

    Field::Element one;
    F.init(one,1);

```

```

for(int i=0;i<stateCount;i++)
{
    // entry in row j and column i is 1 if there is an edge from state i to state j
    for(int k=0;k<alphabet;k++)
        if (stateTransitions[i][k]<stateCount-1)
        {
            Field::Element y;
            F.init(y,0);
            F.add(y,one,AL.getEntry(stateTransitions[i][k],i));
            AL.setEntry(stateTransitions[i][k],i,y);
        }

    // Last row (all 1's)
    AL.setEntry(stateCount-1,i,one);
}

LinBox::Method::SparseElimination M;
solve(Res,AL,BL,M);

for(int i=0;i<stateCount;i++)
    mpq_swap(prob[i].get_mpq_t(),Res[i].get_rep());
}

void printStationaryDistribution(int y)
{
    printf("Stationary distribution for [1:%d]\n",y);
    for (int i=0;i<stateCount;i++)
        if ((i%k)==0)
        {
            printState(y,i);
            gmp_printf(" : %Qd\n",prob[i].get_mpq_t());
        }
}

// Option = event when a frog jumps over a barely nastier frog
// This array holds frequency of all the options (=difference between speeds of successive frogs)
mpq_class optFreq[k+1];

// The following computes option frequency from the stationary distribution
void computeOptFreq(int y)
{
    optFreq[y] = mpq_class(0);
    for (int i=0;i<stateCount;i++)
        for (int c=0;c<alphabet;c++)
            if (transitionEmissions[i][c])
                optFreq[y]+=prob[i];
    optFreq[y]/=alphabet;
}

// Computes constant gamma_W(1), where the expected LCS between a random string of length n
// and the periodic string is gamma_W(1)*n+O(sqrt(n))
//
// Since not all entries optFreq[..] might have been computed yet, this function might return
// "I do not know" together with an upper bound on gamma_W
//
// Input:

```

```

// ymin --- the smallest y for which OptFreq[y] has been computed
// Output:
// true iff either an exact value is computed
// false iff an upper bound is computed
// m is either computed exact value or upper bound
bool estimateExpectedLCS(mpq_class &m, int ymin)
{
    mpq_class left(1,k); // How many periods are left. At start, left = rho/k. We use rho=1; hence left=1/k.
    m=0;

    for(int i=k; i>=ymin; i--)
    {
        if (optFreq[i]>=left)
        {
            m+=i*left;
            return true;
        }
        m += optFreq[i]*i;
        left -= optFreq[i];
    }

    // The best we can hope is that all remaining options are ymin-1
    // in that case we get a match of length m + (ymin-1)*left
    m += (ymin-1)*left;
    return (ymin==1);
}

// modifies periodicWord to the lexicographically next word
// returns true if successful; returns false, if there are no more words
bool nextPeriodicWord()
{
    int i=k-1;
    while ((i>=0)&&(periodicWord[i]!='0'+alphabet-1))
        i--;
    if (i<0) return false;
    periodicWord[i]++;
    while((++i)<k)
        periodicWord[i]='0';
    return true;
}

// returns true if periodicWord is equivalent, under dihedral group, to a lexicographically smaller word
bool wasTested()
{
    // cyclic shifts
    for(int shift=1; shift<k; shift++)
    {
        int pos=0;
        while ((pos<k)&&(periodicWord[pos]==periodicWord[(pos+shift)%k]))
            pos++;
        if ((pos<k)&&(periodicWord[pos]>periodicWord[(pos+shift)%k]))
            return true;
    }
    // reflections
    for(int shift=1; shift<k; shift++)
    {
        int pos=0;
        while ((pos<k)&&(periodicWord[pos]==periodicWord[(k-pos+shift)%k]))
            pos++;
    }
}

```

```

        if ((pos<k)&&(periodicWord[pos]>periodicWord[(k-pos+shift)%k]))
            return true;
    }

    return false;
}

// let f(c) be the number of c's in periodicWord
// the following returns true if f(0)>=f(1)>=...
bool decreasingWeight()
{
    int f[alphabet];
    memset(f,0,sizeof(f));
    for(int i=0;i<k;i++)
        f[periodicWord[i]-'0']++;
    if (balancedOnly)
        for(int c=0;c<alphabet-1;c++)
            if (f[c]!=f[c+1]) return false;

    for(int c=0;c<alphabet-1;c++)
        if (f[c]<f[c+1]) return false;
    return true;
}

// modifies periodicWord to the lexicographically next word that is not cyclically equivalent to one we already tested
// returns true if successful; returns false, if there are no more words
bool nextUntestedWord()
{
    do {
        if (!nextPeriodicWord())
            return false;
    } while (wasTested()||(!decreasingWeight()));
    return true;
}

// y=k-3
//const int Tbl[] = {0,0,0,0,24,500,4500,25725,109760,381024,1134000,2994750};
const int Tbl[] = {0,0,0,9,96,500,1800,5145,12544,27216,54000,99825,174240};

int main()
{
    mpq_class bestExpectedLCS(0,1);
    if (balancedOnly)
        printf("Balanced case. ");
    printf("k = %d\n",k);
    optFreq[k]=mpq_class(1,k*alphabet); // Hand-computed

    for(int y=1;y<k;y++)
        computePossibleFragments(y);

    int wordNum=0;
    do {
        wordNum++;
        printf("Testing %s [%d]\n",periodicWord,wordNum);
        initIs(periodicWord);
        int y=k;
        mpq_class m;
        do {
            computeTransitions(--y);

```

```

computeStationaryDistribution();
// printStationaryDistribution(y);
computeOptFreq(y);
if (estimateExpectedLCS(m,y))
{
    gmp_printf("Expected LCS for %s is %Qd (=%f)\n",periodicWord,m.get_mpq_t(),mpq_get_d(m.get_mpq_t()));
    if (m>bestExpectedLCS)
        bestExpectedLCS=m;
    break;
}
if (m<=bestExpectedLCS)
{
    // The upper bound on gamma_W of this word is no larger than the largest gamma_W seen so far
    break;
}
} while (true);
} while (nextUntestedWord());
printf("%d words\n",wordNum);
}

```

```

compile.sh
#!/bin/bash
# Dependencies: LinBox, IML
g++ -O3 -Wall froglcs.cpp -lgmp -lgivaro -lcblas -llinbox -liml -llapack -o frogs

```

The rational numbers that appear as probabilities in the stationary distribution become large very quickly. For longer words  $W$  we adapted the approach of Lueker [2] to get lower bounds on  $\gamma_W$  using floating-point arithmetic.

Given a Markov chain on a finite space  $\Omega$ , and a function  $f$  on  $\Omega$ , Lueker's approach computes a lower bound on  $\mathbb{E}_{x \in \Omega} f(x)$  for  $x$  drawn from the stationary distribution. For a state  $x$ , denote by  $x^{(t)}$  the random state obtained by starting at  $x$  and making  $t$  steps of the chain. Lueker observed (Observation 2.1 in [2]) that if  $u \in \mathbb{R}^\Omega$  satisfies

$$\mathbb{E}_{x^{(1)}} u(x^{(1)}) + f(x) \geq u(x) + r \quad \text{for every } x \in \Omega,$$

then

$$\mathbb{E} \left[ u(x^{(t)}) + f(x^{(t-1)}) + \dots + f(x^{(1)}) + f(x) \right] \geq u(x) + tr.$$

Since  $x^{(t)}$  converges to the stationary distribution as  $t \rightarrow \infty$  and  $u$  is bounded, this implies that  $\mathbb{E}_{x \in \Omega} f(x) \geq r$ . It does not matter where the vector  $u$  comes from, but in practice a good vector  $u$  can be computed by iterating the map  $u_{\text{new}}(x) = \mathbb{E} [u_{\text{old}}(x^{(1)}) + f(x)]$ .

```

inexactlcs.cpp
#include <stdlib.h>
#include <string.h>
#include <stdio.h>
#include <assert.h>
#include <fcntl.h>
#include <unistd.h>
#include <set>
#include <vector>

const int alphabet=2;
char periodicWord[] = "0110111010010110010001011010";
const bool searchWord = false; // Should we test just one word or search for a word with large gamma_w?
const bool balancedOnly = true; // Should we test only balanced words (those with equally many of each symbol)
const double LCSthreshold = 0.8183; // Abort if we know that the result will be less than this

// Compute period at compile-time

```

```

#define STRLEN(s) ((sizeof(s)/sizeof(s[0]))-1)
static const int k = STRLEN(periodicWord);

// State is a bitmask, where 1 denotes a frog, 0 denotes absence of a frog
typedef unsigned int state;

void printState(state S)
{
    int width=0;
    while (S!=0)
    {
        printf("%d", (int)(S%2));
        S=S/2;
        width++;
    }
    while (width++ < k)
        printf("0");
}

// Poke frogs at positions indexed by the bitmask I
// The bitmask must have 2k bits and be periodic of length k
// Returns the new state; sets "moved" variable to the number of frogs moved
//
// Let S be ...xy...
// Let I be ....z...
// where y & z are i'th position
// then there will be a frog at position i
// iff x&y or (~x)&y&(~z) or (~y)&x is pushed
state poke(state S, state I, int &moved)
{
    moved = 0;
    // Start with a position following an empty spot
    int i=0;
    while (S & (1<<i))
        i++;
    i++;

    // Doing so guarantees that nobody pushes on us from the back
    bool pushed = false;
    state res=0;
    for (int j=0; j<k; j++)
    {
        state mask = 1<<((i+j)%k);
        if (S & mask) // there is frog at position i
        {
            if (pushed)
            {
                moved++;
                res |= mask;
            }
            else if (I & mask) // nobody pushes, but we are excited
                pushed = true;
            else // nobody pushes, and we are unexcited
                res |= mask;
        }
        else // there is no frog at position i
        {
            if (pushed)

```



```

        {
            moved++;
            res |= mask;
        }
        pushed = false;
    }
}

assert(!pushed); // There is no frog that can push at the last position!

return res;
}

// for each alphabet symbol, the set of sets of lillipads that it excites
static state Is[alphabet];

// Initialize Is array from string s that contains '0', '1', etc (up to 'alphabet-1')
void initIs(const char *s)
{
    assert(k==strlen(s));
    memset(Is,0,sizeof(Is));
    for (int p=0;p<k;p++)
    {
        int v=s[p]-'0';
        Is[v]|=1<<p;
    }
    for (int c=0;c<alphabet;c++)
        Is[c]=Is[c]|(Is[c]<<k); // Repeat twice
}

// precomputed middle binomial coefficients
const int middleBinomial[] =
{1, 1, 2, 3, 6, 10, 20, 35, 70, 126, 252, 462, 924, 1716, 3432, 6435, 12870,
 24310, 48620, 92378, 184756, 352716, 705432, 1352078, 2704156, 5200300, 10400600,
 20058300, 40116600, 77558760, 155117520, 300540195, 601080390};

// Compute the binomial coefficients
// Copied from https://stackoverflow.com/questions/24294192/computing-the-binomial-coefficient-in-c
int binom(int n,int k)
{
    assert(n>=k);
    assert(k>=0);
    int ans=1;
    k=k>n-k?n-k:k;
    int j=1;
    for(;j<=k;j++,n--)
    {
        if(n%j==0)
        {
            ans*=n/j;
        }else
        if(ans%j==0)
        {
            ans=ans/j*n;
        }else
        {
            ans=(ans*n)/j;
        }
    }
}

```

```

    return ans;
}

const int maxStates = middleBinomial[k];           // we cannot have more than that many states (likely quite a bit fewer)
static state reachableStates[maxStates];           // states that actually form a strongly connected component (sorted)
static state transitions[maxStates][alphabet];      // transitions[i] contains indices of states that we can jump to from i'th state
//static state movement[maxStates][alphabet];      // how much we moved making those transitions?
static state totalMovement[maxStates];             // totalMovement[i]=sum_c movement[i][c]
int stateCount;                                   // how big is the strongly connected component?

typedef std::set <state, std::greater <state> > stateSet;

// looks for state in feasibleState array, using binary search
int findReachableState(state S)
{
    // We narrow to half-open interval [L,R)
    int L=0;
    int R=stateCount;
    while (L<R)
    {
        int M=(L+R)/2;
        if (S>reachableStates[M])
            L=M+1;
        else if (S<reachableStates[M])
            R=M;
        else
        {
            assert(S==reachableStates[M]);
            return M;
        }
    }
    assert(false);
    return -1;
}

// computes transitions with l frogs
void computeTransitions(int l)
{
    assert(l>0);
    assert(l<k);

    initIs(periodicWord);

    // We need to start in a strongly connected component
    state S = (1<l)-1;
    int moved;
    int B = binom(k,l);

    for (int i=0; i<B; i++)
        S=poke(S, Is[0], moved);

    // Compute the strongly connected component containing S
    stateSet processed, unprocessed;

    unprocessed.insert(S);
    while (!unprocessed.empty())
    {
        S=*unprocessed.begin();

```

```

    for(int c=0;c<alphabet;c++)
    {
        state Snext = poke(S,Is[c],moved);
        if ((unprocessed.count(Snext)==0)&&(processed.count(Snext)==0))
            unprocessed.insert(Snext);
    }
    unprocessed.erase(S);
    processed.insert(S);
}

// Write out everything into nice tables
stateCount = 0;
for (stateSet::reverse_iterator itr = processed.rbegin(); itr!=processed.rend(); ++itr)
    reachableStates[stateCount++]=*itr;

// Write transitions
for(int i=0;i<stateCount;i++)
{
    int totalMove = 0;
    for(int c=0;c<alphabet;c++)
    {
        state Snext=poke(reachableStates[i],Is[c],moved);
        transitions[i][c]=findReachableState(Snext);
        //movement[i][c]=moved;
        totalMove+=moved;
    }
    totalMovement[i]=totalMove;
}

printf("Computed transitions for %d frogs (out %d). There are %d states.\n",l,k,stateCount);
}

// Modifies periodicWord to the lexicographically next word
// returns true if successful; returns false, if there are no more words
bool nextPeriodicWord()
{
    int i=k-1;
    while ((i>=0)&&(periodicWord[i]=='0'+alphabet-1))
        i--;
    if (i<0) return false;
    periodicWord[i]++;
    while(++i<k)
        periodicWord[i]='0';
    return true;
}

/* next lexicographical permutation */
int next_lex_perm(int *a, int n) {
    # define swap(i, j) {t = a[i]; a[i] = a[j]; a[j] = t;}
    int k, l, t;

    /* 1. Find the largest index k such that a[k] < a[k + 1]. If no such
       index exists, the permutation is the last permutation. */
    for (k = n - 1; k && a[k - 1] >= a[k]; k--);
    if (!k--) return 0;

    /* 2. Find the largest index l such that a[k] < a[l]. Since k + 1 is
       such an index, l is well defined */
    for (l = n - 1; a[l] <= a[k]; l--);

```

```

    /* 3. Swap a[k] with a[l] */
    swap(k, l);

    /* 4. Reverse the sequence from a[k + 1] to the end */
    for (k++, l = n - 1; l > k; l--, k++)
        swap(k, l);
    return 1;
# undef swap
}

// Returns true if periodicWord is equivalent to a lexicographically smaller word
// Equivalence refers to cyclically shifting the symbols and permuting alphabet
bool wasTested()
{
    int perm[alphabet];
    for(int i=0; i<alphabet; i++)
        perm[i]='0'+i;

    do {
        // for each cyclic shifts

        for(int shift=1; shift<k; shift++)
        {
            int pos=0;
            while ((pos<k)&&(periodicWord[pos]==perm[periodicWord[(pos+shift)%k]-'0']))
                pos++;
            if ((pos<k)&&(periodicWord[pos]>perm[periodicWord[(pos+shift)%k]-'0']))
                return true;
        }
    } while (next_lex_perm(perm, alphabet));

    return false;
}

// let f(c) be the number of c's in periodicWord
// the following returns true if f(0)>=f(1)>=...
bool decreasingWeight()
{
    int f[alphabet];
    memset(f, 0, sizeof(f));
    for(int i=0; i<k; i++)
        f[periodicWord[i]-'0']++;
    if (balancedOnly)
        for(int c=0; c<alphabet-1; c++)
            if (f[c]!=f[c+1]) return false;

    for(int c=0; c<alphabet-1; c++)
        if (f[c]<f[c+1]) return false;
    return true;
}

// modifies periodicWord to the lexicographically next word that is not cyclically equivalent to one we already tested
// returns true if successful; returns false, if there are no more words
bool nextUntestedWord()
{
    if (!searchWord) return false;
    do {

```

```

    if (!nextPeriodicWord())
        return false;
} while (wasTested() || (!decreasingWeight()));
return true;
}

// Speeds and partial sums of speeds
double S[k], Totals[k];

// Computes LCS using values in the Totals array
// Input
//   maxL indicates what is the largest l for which Totals[l] has been computed
//   in particular maxL = k-1 indicates that all frog's speeds have been computed (except for the minifroggie)
// Output
//   if enough frog speeds were computed, the function return true and sets result to computed LCS
//   if not enough frog speeds were computed, the function returns false and sets result to an upper bound on LCS
bool computeLCS(int maxL, double &result)
{
    S[0]=0;
    for(int l=1;l<k;l++)
        S[l]=Totals[l]-Totals[l-1];

    int CriticalL=0;
    while ((CriticalL<=maxL)&&(S[CriticalL]*k<=1))
        CriticalL++;

    bool exact = ((CriticalL<=maxL)&&(S[CriticalL]*k>1));

    CriticalL--;
    double LCS = 0;
    LCS=Totals[CriticalL];
    LCS+=(k-CriticalL)*(1/((double)k));
    result=LCS;
    return exact;
}

// computes the lower bound on the total speed of first l frogs
// aims to be within error of the upper bound
// (but it is not guaranteed)
double lowerBoundTotalSpeed(int l, double error)
{
    assert(l>0);
    assert(l<k);

    initIs(periodicWord);

    computeTransitions(l);

    double * v[2];
    for (int i=0;i<2;i++)
        v[i] = (double *)calloc(stateCount,sizeof(double));

    int prev=0;
    int next=1;

    double minDiff;
    double maxDiff;

    do {

```

```

minDiff = 100;
maxDiff = -100;

for(int i=0;i<stateCount;i++)
{
    double t=0;
    for (int c=0;c<alphabet;c++)
        t+=v[prev][transitions[i][c]];

    v[next][i]=(totalMovement[i]+t)/alphabet;
    double Diff=v[next][i]-v[prev][i];
    if (Diff<minDiff)
        minDiff=Diff;
    if(Diff>maxDiff)
        maxDiff=Diff;
}
prev = 1-prev;
next = 1-next;
} while (maxDiff-minDiff>error);

for (int i=0;i<2;i++)
    free(v[i]);

return minDiff/k;
}

double lowerBoundLCS(double error)
{
    Totals[0]=0;
    Totals[1]=1/(((double)k*alphabet);
    for (int l=2;l<k;l++)
    {
        Totals[l]=lowerBoundTotalSpeed(l,error);
        double LCS;
        if (computeLCS(l,LCS))
            return LCS;
        if (LCS<LCSthreshold)
            return 0;
    }
    return -1; // Not enough to compute
}

int main()
{
    printf("k = %d\n",k);

    int wordNum=0;
    do {
        wordNum++;
        printf("Testing %s [%d]\n",periodicWord,wordNum);

        double LCS = lowerBoundLCS(0.000005);

        if (LCS>0.815)
            printf("Lower bound on LCS of %s is %f\n",periodicWord,LCS);
    } while (wordNum<10000);
}

```

```
} while (nextUntestedWord());  
  
return 0;  
}
```

The code reports that  $\gamma_W(1) \geq 0.82118$  for  $W = 0110111010010110010001011010$

## References

- [1] Arturs Backurs and Piotr Indyk.  
Edit distance cannot be computed in strongly subquadratic time (unless SETH is false).  
*STOC'15—Proceedings of the 2015 ACM Symposium on Theory of Computing*, 51–58, 2015. [arXiv:1412.0348](https://arxiv.org/abs/1412.0348)
- [2] George S. Lueker.  
Improved bounds on the average length of longest common subsequences.  
*J. ACM*, 56(3):Art. 17, 2009.
- [3] William J. Masek and Michael S. Paterson.  
A faster algorithm computing string edit distances.  
*J. Comput. System Sci.*, 20(1):18–31, 1980.
- [4] Michele Schimd and Gianfranco Bilardi.  
Bounds and estimates on the average edit distance.  
In *String Processing and Information Retrieval* (eds. Nieves R. Brisaboa and Simon J. Puglisi), 91–106, SPIRE 2019.

---

E-mail: [bbukh@math.cmu.edu](mailto:bbukh@math.cmu.edu)

[Back to the homepage](#)
